# Supplementary material for: Provably Robust Blackbox Optimization for Reinforcement Learning
Source: arXiv:1903.02993 source file (2019-07-08)
Supplement: Supplementary file 1 [file appendix.tex]

\section{Appendix}

\subsection{Proof of Theorem \ref{theorem::convergence_robust}}

Let $\nabla F(\theta_t)$ be the real gradient of $F$ at $\theta_t$.

\begin{lemma}
    $F(\theta_t + \delta_t v^{(t)}_j) - F(\theta_t) =  \langle \nabla F(\theta_t), \delta v_j^{(t)} \rangle + \xi_t$ with $|\xi_t| \leq \delta_t^2 d \lambda$. 
\end{lemma}

This follows immediately from a Taylor expansion and the smoothness assumption on $F$. 

\begin{lemma} \label{lemma::closeness_gradient}
For any $t$ if up to $\rho^*$ fraction of the entries of $y_t$ are arbitrarily corrupted, the gradient recovery optimization problem with input $\theta_t$ satisfies:
\begin{equation}
    \| \hat{\nabla}_{RBO} F(\theta_t) - \nabla F(\theta_t) \| \leq \delta_t d \lambda
\end{equation}

Whenever $K \geq  c_1 d$ and with probability $1-\exp\left( -c_2 d  \right)$
\end{lemma}

The proof of Lemma \ref{lemma::closeness_gradient} and the constants $c_1, c_3$ follow the direct application of Theorem 1 in \cite{dwork2007price}.

As a consequence, we can show the first order Taylor approximation of $F$ around $\theta_t$ that uses the true gradient and the one using the RBO gradient are uniformly close:

\begin{lemma}\label{lemma::sup_gradient}
The following bound holds:
For all $\theta_t \in \Theta$:
\begin{equation*}
    \sup_{\theta \in \Theta} | \langle \theta - \theta_t, \hat{\nabla}_{RBO} F(\theta_t)  \rangle - \langle \theta - \theta_t, \nabla F(\theta_t) \rangle | \leq  \mathcal{B} \delta_t d \lambda
\end{equation*}
\end{lemma}

The next lemma provides us with the first step in our convergence bound: 

\begin{lemma}\label{lemma::fundamental_convergence_inequality}
For any $\theta^*$ in $\Theta$, it holds that:
\begin{align*}%\label{eq:fundamental_convergence_lemma}
    2\left( F(\theta^*)  F(\theta_t)   \right) &\leq \frac{ \| \theta_t - \theta^*\|^2_2  - \|\theta_{t+1} - \theta^* \|_2^2 }{\eta_t} \\
    & \quad + \eta_t \left(  \| \nabla F(\theta_t) \| + \delta_t d \lambda\right)^2 \\
    & \quad + 2\mathcal{B}\delta_t d \lambda 
\end{align*}

\end{lemma}

\begin{proof}
%By concavity of $F$ it is true that $\langle \nabla F(\theta_t), \theta^* - \theta_t \rangle \geq F(\theta*) - F(\theta_t)$. 

Recall that $\theta_{t+1}$ is the projection of $u_{t+1}$ to a convex set $\Theta$. And that $u_{t+1} = \theta_t + \eta_t \hat{\nabla}_{RBO} F(\theta_t)$. As a consequence:

\begin{align}
\begin{split}\label{eq::potential_gradient}
    \| \theta_{t+1} - \theta^* \|^2 &\leq  \| \theta_t + \eta_t \hat{\nabla}_{RBO}F(\theta_t) - \theta^* \|^2 \\
    & = \| \theta_t - \theta^* \|^2 + \eta_t^2 \| \hat{\nabla}_{RBO}F(\theta_t) \|^2 \\
    &\quad- 2\eta_t \langle \hat{\nabla}_{RBO}F(\theta_t), \theta^* - \theta_t \rangle 
\end{split}
\end{align}

Lemma \ref{lemma::closeness_gradient} and the triangle inequality imply:
\begin{equation*}
\|\hat{\nabla}_{RBO} F(\theta_t)  \|^2 \leq \left( \| \nabla F(\theta_t) \| + \delta_t d \lambda   \right)^2
\end{equation*}

This observation plus Lemma \ref{lemma::sup_gradient} applied to Equation \ref{eq::potential_gradient} implies:
\begin{align*}
    2\langle \nabla F(\theta_t), \theta^* - \theta_t \rangle  &\leq \frac{ \| \theta_t - \theta^*\|^2_2  - \|\theta_{t+1} - \theta^* \|_2^2 }{\eta_t} \\
    & \quad + \eta_t \left(  \| \nabla F(\theta_t) \| + \delta_t d \lambda\right)^2 \\
    & \quad + 2\mathcal{B}\delta_t d \lambda 
\end{align*}

Since concavity of $F$ implies $F(\theta^* ) - F(\theta_t) \leq  \langle \nabla F(\theta_t), \theta^* - \theta_t \rangle$ the result follows.
\end{proof}

We proceed with the proof of Theorem \ref{theorem::convergence_robust}:

\begin{align}
\begin{split}
    2 \sum_{t=0}^{T-1} \left( F(\theta^*) -  F(\theta_t)   \right) &\leq \sum_{t=0}^{T-1} \frac{ \| \theta_t - \theta^*\|^2_2  - \|\theta_{t+1} - \theta^* \|_2^2 }{\eta_t} \\
    + \sum_{t=0}^{T-1} \eta_t \left( \| \nabla F(\theta_t)  \| + \delta_t d \lambda \right)^2  
    + 2 \mathcal{B}\delta_t d \lambda 
    \leq \sum_{t=0}^{T-1} \|\theta_{t} - \theta* \|^2 \left( \frac{1}{\eta_t} - \frac{1}{\eta_{t-1}} \right) 
    + \sum_{t=0}^{T-1} \eta_t (L+\delta_t d \lambda)^2  + 2 \mathcal{B}\delta_t d \lambda, 
\end{split}    
\end{align}

where we set $\frac{1}{\eta_{-1}} = 0$. the first inequality is a direct consequence of Lemma \ref{lemma::fundamental_convergence_inequality}. The second inequality follows because $\|  \theta_{T} - \theta^* \| \geq 0$ and $\| \nabla F(\theta) \| \leq L$ for all $\theta \in \Theta$.

As long as $\delta_t \leq \frac{L}{d \lambda \sqrt{t+1}}$ and $\eta_t = \frac{\mathcal{B}}{L \sqrt{t+1}}$. We have that:

\begin{equation*}
\sum_{t=0}^{T-1} F(\theta^*) -F(\theta_t) \leq \frac{13}{2}\mathcal{B} L \sqrt{T} %\frac{\mathcal{B} L \sqrt{T}}{2} + 4\mathcal{B} L \sqrt{T} +  2\mathcal{B} L \sqrt{T} 
\end{equation*}

Since $\sum_{t=1}^{T} \frac{1}{\sqrt{t}} \leq 2\sqrt{T}$. This implies the result of Theorem \ref{theorem::convergence_robust}.

% Notice that $\mathcal{B} \leq 2 \mathcal{R}$ \note{get rid of one of this two bounds}. If $\delta_t \leq \frac{L}{\lambda d \sqrt{T}}$ and $\eta = \frac{\mathcal{R}}{2L\sqrt{T}}$ we get the following bound:
% \begin{equation}
%     \sum_{t=0}^{T-1}  \langle \nabla F(\theta_t) ,  \theta^* - \theta_t \rangle \leq 2\mathcal{R} L \sqrt{T} + 4\mathcal{R} L \sqrt{T}= 6 \mathcal{R} L \sqrt{T}.
% \end{equation}

% By concavity of $F$ it is true that $\langle \nabla F(\theta_t) , \theta^* - \theta_t  \rangle \geq  F(\theta^*) - F(\theta_t)$. We conclude that: 
% \begin{equation}
%     \sum_{t=0}^{T-1} \left(F(\theta^*)  -  F(\theta_t) \right) \leq 2\mathcal{R} L \sqrt{T} + 4\mathcal{R} L \sqrt{T}= 6 \mathcal{R} L \sqrt{T}.
% \end{equation}

% Since $\delta_t d \lambda \leq L$ and therefore $L+ \delta_t d \lambda \leq 2L$. The results of Theorem \ref{theorem::convergence_robust} follow.

%%%%%%%%%%%%%%%%%%%%%%%%%%%%%%%%%%
\subsection{Proof of Theorem \ref{theorem::convergence_robust_strongconvex}}

In this section we flesh out the convergence results for robust gradient descent when $F$ is assumed to be Lipschitz with parameter $L$, smooth with parameter $\lambda$ and strongly concave with parameter $\mu$.

\begin{lemma}\label{lemma::fundamental_convergence_inequality_strong}
For any $\theta^*$ in $\Theta$, it holds that:
\begin{equation*}%\label{eq:fundamental_convergence_lemma}
    2\left( F(\theta^*)  F(\theta_t)   \right) \leq \frac{ \| \theta_t - \theta^*\|^2_2  - \|\theta_{t+1} - \theta^* \|_2^2 }{\eta_t} -\mu \| \theta_t - \theta^*\|^2 + \eta_t \left(  \| \nabla F(\theta_t) \| + \delta_t d \lambda\right)^2  + 2\mathcal{B}\delta_t d \lambda 
\end{equation*}

\end{lemma}

\begin{proof}
%By concavity of $F$ it is true that $\langle \nabla F(\theta_t), \theta^* - \theta_t \rangle \geq F(\theta*) - F(\theta_t)$. 

Recall that $\theta_{t+1}$ is the projection of $u_{t+1}$ to a convex set $\Theta$. And that $u_{t+1} = \theta_t + \eta_t \hat{\nabla}_{RBO} F(\theta_t)$. As a consequence:

\begin{align}
\begin{split}\label{eq::potential_gradient}
    \| \theta_{t+1} - \theta^* \|^2 &\leq  \| \theta_t + \eta_t \hat{\nabla}_{RBO}F(\theta_t) - \theta^* \|^2 \\
    & = \| \theta_t - \theta^* \|^2 + \eta_t^2 \| \hat{\nabla}_{RBO}F(\theta_t) \|^2 \\
    &\quad- 2\eta_t \langle \hat{\nabla}_{RBO}F(\theta_t), \theta^* - \theta_t \rangle 
\end{split}
\end{align}

Lemma \ref{lemma::closeness_gradient} and the triangle inequality imply:
\begin{equation*}
\|\hat{\nabla}_{RBO} F(\theta_t)  \|^2 \leq \left( \| \nabla F(\theta_t) \| + \delta_t d \lambda   \right)^2
\end{equation*}

This observation plus Lemma \ref{lemma::sup_gradient} applied to Equation \ref{eq::potential_gradient} implies:
\begin{align*}
    2\langle \nabla F(\theta_t), \theta^* - \theta_t \rangle  &\leq \frac{ \| \theta_t - \theta^*\|^2_2  - \|\theta_{t+1} - \theta^* \|_2^2 }{\eta_t} \\
    & \quad + \eta_t \left(  \| \nabla F(\theta_t) \| + \delta_t d \lambda\right)^2 \\
    & \quad + 2\mathcal{B}\delta_t d \lambda 
\end{align*}

Since strong concavity of $F$ implies $F(\theta^* ) - F(\theta_t) \leq  \langle \nabla F(\theta_t), \theta^* - \theta_t \rangle - \frac{\mu}{2} \|\theta_t - \theta^* \|^2$ the result follows.
\end{proof}

The proof of Theorem \ref{theorem::convergence_robust_strongconvex} follows from it. Indeed, we have:

\begin{align*}
    2 \sum_{t=0}^{T-1} \left( F(\theta^*) -  F(\theta_t)   \right) &\leq \sum_{t=0}^{T-1} \frac{ \| \theta_t - \theta^*\|^2_2  - \|\theta_{t+1} - \theta^* \|_2^2 }{\eta_t} -\mu \| \theta_t - \theta^*\|^2 + \sum_{t=0}^{T-1} \eta_t \left( \| \nabla F(\theta_t)  \| + \delta_t d \lambda \right)^2  + 2 \mathcal{B}\delta_t d \lambda \\
    &\leq \underbrace{\sum_{t=0}^{T-1} \|\theta_{t} - \theta* \|^2 \left( \frac{1}{\eta_t} - \frac{1}{\eta_{t-1}} - \mu \right) }_{I} + \sum_{t=0}^{T-1} \eta_t (L+\delta_t d \lambda)^2  + 2 \mathcal{B}\delta_t d \lambda 
\end{align*}

Where we set $\frac{1}{\eta_{-1}} = 0$. the first inequality is a direct consequence of Lemma \ref{lemma::fundamental_convergence_inequality_strong}. The second inequality follows because $\|  \theta_{T} - \theta^* \| \geq 0$ and $\| \nabla F(\theta) \| \leq L$ for all $\theta \in \Theta$. Since $\eta_t = \frac{1}{\mu*(t+1)}$, $\frac{1}{\eta_t} - \frac{1}{\eta_{t-1}} = \mu$ for all $t= 0, \cdots , T-1$ the term labeled I in the inequality above vanishes.

As long as $\delta_t \leq \frac{L^2}{d \mathcal{B} \mu \lambda(t+1)}$ we have that

\begin{equation*}
\sum_{t=0}^{T-1} F(\theta^*) -F(\theta_t) \leq \frac{6 L^2}{\mu}(1+\log(T)) 
\end{equation*}

Since $\sum_{t=1}^{T} \frac{1}{t} \leq 1 + \log(T)$. This implies the result of Theorem \ref{theorem::convergence_robust_strongconvex}.

\subsection{More Experimental Results}

We present here more experimental results that we did not include in the main body of the paper. These results are presented in: Fig. \ref{fig:mix_1}, Fig. \ref{fig:swimmer-30-40} and Fig. \ref{fig:swimmer-halfcheetah-mean}.

\begin{figure}[!t]
\begin{minipage}{1.0\textwidth}
	\subfigure[$\mathrm{HalfCheetah}$-noiseless]{\includegraphics[keepaspectratio, width=0.45 \textwidth]{plots/halfcheetah-d1.png}}
	\subfigure[$\mathrm{CMC}$-noiseless]{\includegraphics[keepaspectratio, width=0.45\textwidth]{plots/cmc.png}}
\end{minipage}
	\caption{Left subfigure: as in Figure \ref{fig:swimmer-no-noise}, but for $\mathrm{HalfCheetah}$ environment and $800$ iterations of the algorithm. $\mathrm{LP}$-$\mathrm{full}$-$\mathrm{ort}$ corresponds to the $\mathrm{RBO}$ method with $p=1, \alpha=0$ and gaussian orthogonal vectors taken as sensing directions. Right subfigure: as in Figure \ref{fig:swimmer-no-noise}, but for $\mathrm{Continuous}$ $\mathrm{Mountain}$ $\mathrm{Car}$ environment. $\mathrm{LP}$ stands for the $\mathrm{RBO}$ with $p=1, \alpha = 0$ and the number of samples per iteration $k=\frac{d}{2}$, where $d$ is a dimensionality of a gradient vector. We see that $\mathrm{RBO}$ achieves higher rewards and learns faster, even though it is also characterized by a larger variance.}
	\label{fig:mix_1} 
\end{figure}

\begin{figure}[!t]
\begin{minipage}{1.0\textwidth}
	\subfigure[$\mathrm{Swimmer}$-$0.3$]{\includegraphics[keepaspectratio, width=0.45\textwidth]{plots/swimmer_03.png}}
	\subfigure[$\mathrm{Swimmer}$-$0.4$]{\includegraphics[keepaspectratio, width=0.45\textwidth]{plots/swimmer_04.png}}	
\end{minipage}
	\caption{Left subfigure: as in Fig. \ref{fig:swimmer-10}, but this time $30\%$ of all the measurements were arbitrarily corrupted. Right subfigure: as in Fig. \ref{fig:swimmer-10}, but this time $40\%$ of all the measurements were arbitrarily corrupted.}
	\label{fig:swimmer-30-40} 
\end{figure}

\begin{figure}[!t]
\begin{minipage}{1.0\textwidth}
	\subfigure[$\mathrm{Swimmer}$-mean curve]{\includegraphics[keepaspectratio, width=0.45\textwidth]{Jack_Sam/SWIMMER/SW_20noise_h16_notOrt_k1_Average.png}}
	\subfigure[$\mathrm{HalfCheetah}$-shadow]{\includegraphics[keepaspectratio, width=0.45\textwidth]{Jack_Sam/HLF_CHTAH/HC_0noise_h32_notOrt_k2_Mean.png}}	
\end{minipage}
	\caption{Left subfigure: mean training curve, $\mathrm{max}$ and $\mathrm{min}$ values for $20$ different seeds on the $\mathrm{Swimmer}$ environment, with the use of $\mathbf{RBO}$ with $p=1, \alpha=0$ (LP decoding) and $20\%$ of measurements arbitrarily corrupted. Right subfigure: as in the left subfigure, but for the $\mathrm{HalfCheetah}$ environment and in the noiseless setting.}
	\label{fig:swimmer-halfcheetah-mean} 
\end{figure}

\subsection{Further Experimental Details}

Below we include additional information regarding the implementation and performance of the $\mathrm{RBO}$ algorithm, in particular for the setting with $p=1, \alpha=0$ (LP decoding).

\paragraph{Optimization:} Policy updates were conducted with the Adam Optimizer, with a fixed learning rate. We did not use any heuristics such as fitness shaping.

\paragraph{Consistency of Results:} We ran $20$ different seeds for each of $\mathrm{Continuous}$ $\mathrm{Mountain}$ $\mathrm{Car}$, $\mathrm{Pendulum}$ and $\mathrm{Swimmer}$.

\newpage

\bigskip
\begin{tabular}{ C{0.8in}  *3{C{.6in}} }\toprule[1.5pt]
\bf $\mathbf{Setting}$ & \bf $\mathrm{Continuous}$ $\mathrm{Mountain}$ $\mathrm{Car}$ & \bf $\mathrm{Pendulum}$ & \bf $\mathrm{Swimmer}$ \\\midrule
Noiseless   & $100\%$ & $100\%$ & $75\%$ \\
Noisy  & $100\%$ & $95\%$ & $80\%$ \\
\bottomrule[1.25pt]
\end {tabular}\par
\smallskip
\small{Table 2: The percentage of seeds which achieved a good reward, in noiseless and noisy settings, for the $\mathrm{RBO}$ algorithm with $p=1, \alpha=0$. For thresholds, we took $90$ for $\mathrm{Continuous}$ $\mathrm{Mountain}$ $\mathrm{Car}$, $-5000$ for $\mathrm{Pendulum}$ and $300$ for $\mathrm{Swimmer}$. These levels were chosen based on scores which typically led to good policies in practice.}

\subsection{Further experimental details}
